# Supplementary material for: Mesh Strikes Back: Fast and Efficient Human Reconstruction from RGB videos
Source: arXiv:2303.08808 source file (2023-03-15)
Supplement: Supplementary file 1 [file supp.tex]

\section{Supplementary Material}

In this section, we provide more implementation details, ablations, and qualitative examples.

\begin{table*}[t!]
   \centering 
   \begin{tabularx}{\linewidth}{XYYYYY} \toprule
   \multicolumn{6}{c}{\textbf{Training time (in mins)}} \\ \midrule
    \textbf{Subject} & \textbf{Ours} & \textbf{AnimNeRF} & \textbf{Neuralbody} & \textbf{people-snapshot} & \textbf{SMPLPix} \\ \midrule
    \textbf{male-3-casual} & 44.74 & 847.18 & 708.47 & 560.28 & 463.21 \\
    \textbf{male-4-casual} & 43.08 & 763.30 & 705.19 & 660.53 & 707.16 \\
    \textbf{female-3-casual} & 46.80 & 823.01 & 1332.80 & 531.07 & 451.68 \\
    \textbf{female-4-casual} & 38.63 & 643.58 & 1334.65 & 453.77 & 359.00 \\ \midrule
    \multicolumn{6}{c}{\textbf{GPU requirements (in MiB)}} \\ \hline
    \textbf{male-3-casual} & 5919 & 47822 & 3761 & - & 14083 \\
    \textbf{male-4-casual} & 5919 & 47822 & 3721 & - & 14083 \\
    \textbf{female-3-casual} & 5619 & 45620 & 3449 & - & 14083 \\
    \textbf{female-4-casual} & 5515 & 47822 & 4051 & - & 14083 \\ \bottomrule
   \end{tabularx}
    \caption{\textbf{Individual training time and compute analysis}: Our method has a very low overall compute and training time requirements compared to other methods.}
   \label{tab:trainingtime}
\end{table*}

\subsection{Implementation details}
In this section, we describe more implementation details for the method.
We implement the entire framework in PyTorch \cite{pytorch}.
For people-snapshot dataset, we choose $\lambda_{\text{RGB}} = 4$, $\lambda_{\text{Sil}} = 4$, $\lambda_{\text{kps}} = 0.01$, $\lambda_{NC} = 0.5$, $\lambda_{FA} = 2.5$ for all subjects.
For ZJU dataset, we change $\lambda_{\text{Sil}} = 6$ and keep everything else the same for all subjects.
For self-recon, we use $\lambda_{\text{kps}} = 1.0$ since we have more accurate keypoints for the synthetic model.
For the hash encoding representation, we choose $N_{min} = 16, N_{max} = 1024$, $T = 2^{19}$ and $L = 16$.
We refer the reader to \cite{mueller2022instantngp} for more information on the hyperparameters of the hash encoding representation. 
For human shape model, we use the SMPL \cite{SMPL:2015} model with 6890 vertices and 13776 faces in all experiments unless mentioned otherwise.
We use the Adam \cite{kingma2014adam} optimizer with learning rate of $0.001$ for all parameters and $0.01$ for the per-face base RGB color.
We render 512x512 images in all experiments, and train all models on a single GeForce RTX 3090 GPU.

\begin{table*}[t!]
    \centering
    \begin{tabular}{lcccccc} \toprule
    \multirow{2}{*}{\textbf{Subject}} & \multicolumn{2}{c}{\textbf{PSNR} $\uparrow$} & \multicolumn{2}{c}{\textbf{SSIM} x100 $\uparrow$} & \multicolumn{2}{c}{\textbf{LPIPS} x100 $\downarrow$} \\
    & \textbf{Texels}  & \textbf{Ours} & \textbf{Texels}  & \textbf{Ours} & \textbf{Texels}  & \textbf{Ours} \\
    \midrule
    {male-3-casual} & 28.49 & \textbf{29.40} & \textbf{96.24} & \textbf{96.24} & 2.73 & \textbf{2.65} \\
    {male-4-casual} & 25.98 & \textbf{26.31} & 93.97 & \textbf{94.27} & 5.71 & \textbf{5.30} \\
    {female-3-casual} & {26.39} & \textbf{27.25} & {96.17} & \textbf{96.21} & {3.55} & \textbf{3.47} \\
    {female-4-casual} & 28.63 & \textbf{29.61} & 96.59 & \textbf{96.61} & 2.67 & \textbf{2.42} \\
    \bottomrule
    \end{tabular}
    \caption{\textbf{Ablation on texture representation}: We obtain good improvements in PSNR for novel view reconstruction across all subjects in people-snapshot dataset.
    }
    \label{tab:texnet}
\end{table*}

\subsection{Novel view reconstruction}
\label{sec:novelviewsupp}
We provide more qualitative examples of novel view reconstruction in the people-snapshot dataset in Figures \ref{fig:novelview-f4c}, \ref{fig:novelview-f3c}, \ref{fig:novelview-m3c}, \ref{fig:novelview-m4c}. 
Across all subjects, we see a common pattern - SMPLpix is unable to render accurate renderings for novel views.
% This is because \rohitcomment{need to add Ganesh's writeup.}.
This is because SMPLpix operates on a per-frame basis, so there is no consistency enforced among frames in terms of shape or deformations.
This leads to SMPLpix producing inconsistent renderings from different views.
Our results are consistent with those presented in \cite{chen:arxiv2021:animner}.  
VideoAvatar is unable to recover accurate geometry - in case of \textbf{f4c}, it is unable to recover the hair bun and loose clothing near the shoulders.
The face of subjects \textbf{f3c} and \textbf{f4c} are significantly distorted, in comparison to AnimNeRF and our method.
VideoAvatar also leaves all fingers open as in the default SMPL model, whereas all other models chose the hands (including our method).
% All subjects have their hands open in the VideoAvatar results, whereas every other method (including ours) is able to model the closed hands.
% the hair bun and loose clothing near the shoulders are modelled incorrectly in \textbf{f4c}, no wrinkles in the jeans of \textbf{m3c}, incorrect head shape of \textbf{f3c}.
Neuralbody starts to deteriorate in quality as soon as the novel view pointcloud distribution slightly deviates from the training pointcloud distribution.
This renders neuralbody a bad baseline for generalization since it overly fits to the training images, similar to SMPLpix.
AnimNeRF renders very accurate novel view reconstructions, but has occasional cloud artifacts (in \textbf{f3c}) which amplifies in novel pose reconstruction.
Moreover, AnimNeRF takes a lot of compute and needs a long time to train.
Note that our method is based on a mesh representation only, but is virtually indistinguishable from AnimNeRF.

Qualitative examples for ZJU dataset is shown in Figure ~\ref{fig:novelview-zju}.
Subjects in the ZJU dataset bring additional complexity in terms of rapidly deforming wrinkles in clothes, variable diffuse light components from different views (cameras), and arbitrary poses with significant deviation from the A-pose.
Unlike the people-snapshot dataset, this poses a challenge to our method, since a point on the mesh receives conflicting colors from different views. 
Therefore, we observe slight jaggedness in our learnt texture, which reflects in a lower SSIM (Table 2 in the main paper).
However, our method has very competitive PSNR and LPIPS values when compared to HumanNeRF, and significantly surpasses other methods.
The only noticably worse reconstruction is observed for Subject 393 and 387, which occurs due to rapidly deforming winkles in the hoodie, which leads to rapid change in shading.
In spite of these challenging conditions, our method recovers a very accurate mesh.
Future work can look into adopting deformations and variable lighting as part of the formulation.

\subsection{OOD Novel pose reconstruction}
\label{sec:novelposesupp}
In addition to novel view reconstruction, we analyse the quality of out-of-distribution novel pose rendering in the people-snapshot dataset.
Results are shown in Fig.~\ref{fig:novelpose-f3c}, ~\ref{fig:novelpose-f4c},~\ref{fig:novelpose-m3c},~\ref{fig:novelpose-m4c}.
SMPLpix has unsurprisingly very similar performance as novel view reconstruction.
% , due to reasons discussed in Sec. \ref{sec:novelviewsupp}.
Neuralbody suffers the most because the pointcloud distribution of novel poses deviates significantly from the pointcloud distribution of training poses, leading to extreme quality distortion.
In many cases, the face is not recoverable at all.
In AnimNeRF, we observe cloud artifacts for all subjects, even when the AnimNeRF is trained with background regularization (this is the default setting).
This can happen when certain points in the canonical space (\eg near the armpits and thighs) are not queried during training at all, owing to occlusion from \textit{every} input view.
These points will have undefined occupancy and color, which we observe in novel pose renderings.
Mesh-based methods \ie VideoAvatar and our method don't have this problem, and we do not see artifacts.
However, VideoAvatar has inaccurate geometry which leads to unrealistic faces during texture optimization, while ours look more perceptually accurate (similar to AnimNeRF).

\subsection{Geometry reconstruction}
We qualitatively evaluate the geometry recovered by different methods in people-snapshot and ZJU datasets.
Results are shown in Fig.~\ref{fig:geom} and Fig.~\ref{fig:geom2}.
Note that our mesh can capture loose clothing and voluminous hair better compared to VideoAvatar which uses the same underlying mesh.
Our mesh looks very similar to the meshes recovered by AnimNeRF, which have recovered meshes with the number of vertices being an order of magnitude more than that of our model.
For ZJU Mocap dataset, our method clearly recovers more intricate details, with the same mesh representation.
To our knowledge, HumanNeRF does not recover an explicit geometry.

\subsection{Timing analysis of AnimNeRF}
AnimNeRF achieves state-of-the-art results on rendering and geometry reconstruction.
However, it is prohibitively expensive both in terms of time and compute.
One might argue that this is because of the NeRF implementation used, and can be sped up considerably using faster NeRF optimizations ~\cite{yu_and_fridovichkeil22plenoxels,mueller2022instantngp,Garbin21FastNeRF}.
We implement and evaluate AnimNeRF with the InstantNGP ~\cite{mueller2022instantngp} representation, which has shown tremendous benefits in static NeRFs.
However, in this case we observe that the main bottleneck of AnimNeRF is the KNN operation to `undo' the rays from the observation space to canonical space.
A profiling analysis of the training loop components (Fig~\ref{fig:timingnerf}a) reveals that the KNN operation takes significantly longer than the backward pass. 
Fig.~\ref{fig:timingnerf}b shows that using InstantNGP has no effect on quantitative metrics, and only has a slight edge in terms of training time.
This implies that a faster pipeline has to replace the KNN step with an efficient and appropriate way to canonicalize the representation.
Our method combines a mesh representation and differentiable rendering using rasterization to perform fast and efficient canonicalization.
A more finegrained analysis of training time and compute requirements for people-snapshot are provided in Table ~\ref{tab:trainingtime}.

\begin{table*}[t!]
    \centering
    \begin{tabular}{lcccccc} \toprule
    \multirow{2}{*}{\textbf{Subject}} & \multicolumn{2}{c}{\textbf{PSNR} $\uparrow$} & \multicolumn{2}{c}{\textbf{SSIM} $\uparrow$} & \multicolumn{2}{c}{\textbf{LPIPS} $\downarrow$} \\
    & \textbf{One stage}  & \textbf{Two stage} & \textbf{One stage}  & \textbf{Two stage} & \textbf{One stage}  & \textbf{Two stage} \\
    \midrule
    {male-3-casual} & 25.67 & \textbf{29.40} & .9469 & \textbf{.9624} & .0400 & \textbf{.0265} \\
    {male-4-casual} & 22.42 & \textbf{26.31} & .9167 & \textbf{.9427} & .0842 & \textbf{.0530} \\
    {female-3-casual} & \textbf{27.56} & 27.25 & \textbf{.9636} & .9621 & \textbf{.0338} & .0347 \\
    {female-4-casual} & 29.52 & \textbf{29.61} & .9653 & \textbf{.9661} & .0244 & \textbf{.0242} \\
    \bottomrule
    \end{tabular}
    \caption{\textbf{Ablation on two-stage training}: Note that our method produces accurate reconstruction across all 4 subjects, but one-stage training collapses for male subjects with uneven textures and complex shapes.
    This is due to the moving targets problem, where the gradients for texture and mesh deformation hinder each other's learning.
    Even for subjects \textbf{f3c} and \textbf{f4c}, qualitative results in Fig.~\ref{fig:onestage} show that two-stage training is robust.
    }
    \label{tab:onestage}
\end{table*}

\subsection{Ablation on two stage training}
% We also compare the effect of two stage training.
% To compare the effect of two-stage training, we also train our mesh parameters and texture network with a one-stage training approach.
To demonstrate why two-stage training is necessary, we train our model with the one-stage training approach on people-snapshot.
In this case, all parameters (human body and texture network parameters) are optimized simultaneously.
We show some qualitative and quantitative results in Table ~\ref{tab:onestage} and Fig. ~\ref{fig:onestage}. 
The \textit{moving target} problem is more prominent in subjects \textbf{m4c} and \textbf{f4c} where the textures are highly distorted.
This problem necessitates a two-stage training paradigm.
GIFs of recovered geometry are provided in the Supplementary Video.

% It is important to note that although one-stage training is able to capture texture well in uniformly textured regions, it morphs the geometry in unnatural ways. 
% This makes the one-stage training paradigm brittle, and we therefore adopt a two-stage approach in this work.

\subsection{Effect of adaptive texture representation}
We also compare our texture representation with a texture memory representation, which is non-adaptive.
We choose the texel size to match the size of encoder representation, which corresponds to a texel size of 6.
All the other training parameters are the same, except the texture representation.
Quantitative novel view results are shown in Table \ref{tab:texnet}.

\subsection{Performance of VideoAvatar on ZJU}
An initial run of VideoAvatar~\cite{alldieck:cvpr2018:peoplesnap} on ZJU dataset fails to converge. 
We identify a few reasons: the A-pose prior is strong, and the prior does not hold in the ZJU dataset at all.
Moreover, ZJU dataset also provides an external rotation and translation parameter for each frame that is independent of the SMPL parameters ~\cite{zjulink}.
This leads to a bad initialization for the pose in each frame.
Moreover, the camera is hardcoded, making it difficult to incorporate multi-view optimization.
To enable a fair comparison, we make the following changes:
first, we multiply the final rotation and translation parameters 
into the extrinsics matrix to provide a good initialization for the camera.
Second, we change the SMPL pose regressor and keypoint losses to use the 2D keypoints provided in the ZJU dataset.
Third, we change the pose prior for each frame to be close to pose parameters provided in the dataset. 
We observe that even with a good initialization, the optimization fails to cover significant portions of the visual hull.
These gross errors in coverage of the visual hull results in inaccurate textures propagated to the mesh, and consequently an inaccurate reconstruction and geometry.
We provide Supplementary Videos of the optimization process to ensure that we perform a fair comparison for VideoAvatar in the ZJU dataset. 

%%%%%%%%%%%%%%%%%%%%%%%%%% 
% Anim NeRF time analysis
%%%%%%%%%%%%%%%%%%%%%%%%%% 
\begin{figure*}
\centering
% Pie chart
\begin{minipage}{0.33\linewidth}
\centering
\includegraphics[width=\linewidth]{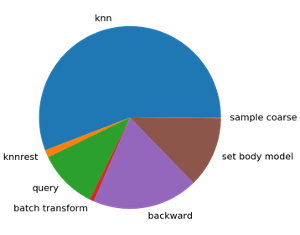}
\end{minipage}
% 
% Time for training
\begin{minipage}{0.66\linewidth}
\centering
    \begin{tabular}{lrr} \toprule
    &  \textbf{AnimNeRF} & \textbf{AnimNeRF + InstantNGP} \\
    \midrule
    \textbf{PSNR} & 29.37 & 29.30 \\
    \textbf{SSIM} x100 & 97.03 & 96.89 \\
    \textbf{LPIPS} x100 & 1.68 & 1.64 \\
    \textbf{Training time (hrs)} & 14.85 & 12.95 \\
    \bottomrule
    \end{tabular}
\end{minipage}
\begin{minipage}{\linewidth}
\begin{minipage}{0.33\linewidth}
\centering (a)
\end{minipage}
\begin{minipage}{0.66\linewidth}
\centering (b)
\end{minipage}
\end{minipage}
\caption{\textbf{Timing analysis on AnimNeRF.}
(a) shows the profiling of the training iteration and its components.
Note that the bottleneck here is not the NeRF but the canonicalization of rays using KNN, which cannot be alleviated using Faster NeRF variants.
(b) compares the base AnimNeRF and AnimNeRF with InstantNGP ~\cite{mueller2022instantngp} representation. Note that there is no difference in any quantitative metrics for novel view reconstruction, and speedups in training time is not significant either.}
\label{fig:timingnerf}
\end{figure*}

\begin{figure*}
    \centering
    \includegraphics[width=0.95\linewidth]{figures/onestage.png}
    \caption{\textbf{One-stage v/s two-stage novel view reconstruction}: Top row shows novel view reconstructions for one-stage training, and bottom row is for two-stage training (ours).
    Note that one-stage collapses for subjects \textbf{m3c} and \textbf{m4c}, leading to distorted geometry (highlighted in red).
    For \textbf{f3c} and \textbf{f4c} it has minor color and pose artifacts. Videos of meshes are provided in Supplementary GIFs.
    }
    \label{fig:onestage}
\end{figure*}

%%% Geometry
\begin{figure*}
    \centering
    \includegraphics[width=0.7\linewidth]{figures/geom_details/geom1.png}
    \includegraphics[width=0.7\linewidth]{figures/geom_details/geom2.png}
    \includegraphics[width=0.7\linewidth]{figures/geom_details/geom3.png}
    \includegraphics[width=0.7\linewidth]{figures/geom_details/geom4.png}
    \caption{\textbf{Geometry reconstruction on people-snapshot dataset}: VideoAvatar fails to capture intricate details of the subject, and preserves a lot of the initial details of the underlying SMPL mesh, which do not reflect the subject's true geometry.
    Our model recovers geometry that is very similar to AnimNeRF's recovered geometry, showing that it is possible to directly optimize a mesh to recover accurate geometry.}
    \label{fig:geom}
\end{figure*}
\begin{figure*}
    \centering
    \includegraphics[width=\linewidth]{figures/zju-geom.png}
    \caption{\textbf{Geometry reconstruction on ZJU dataset}: 
    Top row shows reconstructions from VideoAvatar, bottom row shows reconstructions from our method.
    Compared to VideoAvatar, our method extracts more intricate geometry, including loose clothing, voluminous hair, etc. with the same mesh representation.
    To our knowledge, HumanNeRF does not recover explicit geometry.
    }
    \label{fig:geom2}
\end{figure*}

% novel view
\begin{figure*}
    \centering
    \includegraphics[width=0.9\linewidth]{figures/novelview/female4c-nv3.png}
    \includegraphics[width=0.9\linewidth]{figures/novelview/female4c-nv2.png}
    \includegraphics[width=0.9\linewidth]{figures/novelview/female4c-nv1.png}
    \caption{\textbf{Novel view reconstruction (female-4-casual)}. Note that SMPLpix fails to recover accurate face and clothing details.
    VideoAvatar doesn't model the shape correctly and has visibly different reconstruction than the others.
    Moreover, identity of the subject is distorted in VideoAvatar. 
    NeuralBody introduces `bubble artifacts` near the head and limbs. 
    Our method and AnimNeRF output accurate geometry and very detailed texture. }
    \label{fig:novelview-f4c}
\end{figure*}

\begin{figure*}
    \centering
    \includegraphics[width=0.9\linewidth]{figures/novelview/female3c-nv1.png}
    \includegraphics[width=0.9\linewidth]{figures/novelview/female3c-nv2.png}
    \includegraphics[width=0.9\linewidth]{figures/novelview/female3c-nv3.png}
    \caption{\textbf{Novel view reconstruction (female-3-casual)}. }
    \label{fig:novelview-f3c}
\end{figure*}

\begin{figure*}
    \centering
    \includegraphics[width=0.9\linewidth]{figures/novelview/male3c-nv1.png}
    \includegraphics[width=0.9\linewidth]{figures/novelview/male3c-nv2.png}
    \includegraphics[width=0.9\linewidth]{figures/novelview/male3c-nv3.png}
    \caption{\textbf{Novel view reconstruction (male-3-casual)}. }
    \label{fig:novelview-m3c}
\end{figure*}

\begin{figure*}
    \centering
    \includegraphics[width=0.9\linewidth]{figures/novelview/male4c-nv2.png}
    \includegraphics[width=0.9\linewidth]{figures/novelview/male4c-nv3.png}
    \includegraphics[width=0.9\linewidth]{figures/novelview/male4c-nv1.png}
    \caption{\textbf{Novel view reconstruction (male-4-casual)}. }
    \label{fig:novelview-m4c}
\end{figure*}

\begin{figure*}
   \centering 
   \includegraphics[width=0.7\linewidth]{figures/novelview/zju-377.png}
   \includegraphics[width=0.7\linewidth]{figures/novelview/zju-392.png}
   \includegraphics[width=0.7\linewidth]{figures/novelview/zju-394.png}
   \caption{\textbf{Novel view reconstruction on ZJU dataset}: From left to right- SMPLPix, VideoAvatar, Neuralbody, HumanNeRF, Ours }
   \label{fig:novelview-zju}
\end{figure*}

\begin{figure*}
    \centering
    \includegraphics[width=0.9\linewidth]{figures/novelpose/f3-26.png}
    \includegraphics[width=0.9\linewidth]{figures/novelpose/f3-23.png}
    \includegraphics[width=0.9\linewidth]{figures/novelpose/f3-02.png}
    \caption{\textbf{Novel pose reconstruction (female-3-casual)}.}
    \label{fig:novelpose-f3c}
\end{figure*}

\begin{figure*}
    \centering
    \includegraphics[width=0.9\linewidth]{figures/novelpose/f4-36.png}
    \includegraphics[width=0.9\linewidth]{figures/novelpose/f4-20.png}
    \includegraphics[width=0.9\linewidth]{figures/novelpose/f4-07.png}
    \caption{\textbf{Novel pose reconstruction (female-4-casual)}.}
    \label{fig:novelpose-f4c}
\end{figure*}

\begin{figure*}
    \centering
    \includegraphics[width=0.9\linewidth]{figures/novelpose/m3-18.png}
    \includegraphics[width=0.9\linewidth]{figures/novelpose/m3-32.png}
    \includegraphics[width=0.9\linewidth]{figures/novelpose/m3-15.png}
    \caption{\textbf{Novel pose reconstruction (male-3-casual)}.}
    \label{fig:novelpose-m3c}
\end{figure*}

\begin{figure*}
    \centering
    \includegraphics[width=0.9\linewidth]{figures/novelpose/m4-30.png}
    \includegraphics[width=0.9\linewidth]{figures/novelpose/m4-28.png}
    \includegraphics[width=0.9\linewidth]{figures/novelpose/m4-13.png}
    \caption{\textbf{Novel pose reconstruction (male-4-casual)}.}
    \label{fig:novelpose-m4c}
\end{figure*}
